# Supplementary material for: Building Self-Evolving Agents via Experience-Driven Lifelong Learning: A Framework and Benchmark
Source: arXiv:2508.19005 source file (2026-01-26)
Supplement: Supplementary file 1 [file appendix_main.tex]

\documentclass{article}
\usepackage{amsmath}
\usepackage{amssymb}
\usepackage{amsthm}
\usepackage{geometry}
\usepackage{enumitem}
\usepackage{booktabs} 
\usepackage{graphicx} % 用于 \resizebox
\usepackage{multirow} % 用于 \multirow
\usepackage{booktabs} % 用于 \toprule, \midrule, \bottomrule
\usepackage[utf8]{inputenc}
\usepackage{tabularx}
\geometry{a4paper, margin=1in}

% --- 这是修复后的新代码 ---
\usepackage{tcolorbox}
\usepackage{listings} % 1. 额外加载 listings 宏包
\tcbuselibrary{breakable, listings} % 2. 将 tcolorbox 的库从 verbatim 改为 listings

% 3. 使用 \newtcblisting 重新定义 promptbox 环境
\tcbuselibrary{listings} % 加载 tcolorbox 的 listings 库
% --- 1. 用于普通段落文字的盒子 ---
\newtcolorbox{textBox}[1][]{
  colback=gray!5,
  colframe=gray!60!black,
  fonttitle=\bfseries,
  colbacktitle=gray!85!black,
  title=#1,
  breakable
}

% --- 2. 用于工具/代码声明的盒子 ---
\newtcblisting{promptbox}[1][]{
  colback=gray!5,
  colframe=gray!60!black,
  fonttitle=\bfseries,
  colbacktitle=gray!85!black,
  title=#1,
  breakable,
  listing only,
  listing options={
    basicstyle=\ttfamily\small,
    breaklines=true,
    columns=fullflexible
  }
}
\theoremstyle{definition}

\begin{document}

\title{Building a Self-Evolving Agent via Experience-Driven Lifelong Learning: A Framework and Benchmark}
\author{}
\date{}
-

\input{appendix}
\end{document}
